# Supplementary material for: MATE-Pred: Multimodal Attention-based TCR-Epitope interaction Predictor
Source: arXiv:2401.08619 source file (2023-12-05)
Supplement: Supplementary file 1 [file appendix.tex]

\begin{document}%--------------------------------

\setcounter{table}{0}
\renewcommand{\thetable}{A\arabic{table}}
\vspace{-4mm}
\begin{table}[!ht]
\caption{Ligand Physicochemical descriptors details.}
\centering
\begin{tabular}{|c|c|}
\hline
\textbf{Name} & \textbf{Dimensions} \\ \hline
BLOSUM Indices & 10 \\ \hline
Cruciani Properties & 3 \\ \hline
FASGAI vectors & 6 \\ \hline
Kidera factors & 10 \\ \hline
MS-WHIM scores & 3 \\ \hline
PCP properties & 5 \\ \hline
ProtFP descriptors & 8 \\ \hline
Sneath vectors & 4 \\ \hline
ST-scales & 8 \\ \hline
T-scales & 5 \\ \hline
VHSE-scales & 8 \\ \hline
Z-scales & 5 \\ \hline
\hline
Total length  & 75 \\  \hline                                               
\end{tabular}
\label{table:physicochemical_list}
\end{table}

\begin{table}[!ht]
\caption{Ligand Global Properties details.}
\centering
\begin{tabular}{|c|c|}
\hline
\textbf{Name} & \textbf{Dimensions} \\ \hline
Aliphatic Index & 1 \\ \hline
Autocorrelation & 1 \\ \hline
Autocovariance & 1 \\ \hline
Boman Index & 1 \\ \hline
Lehninger Charge & 1 \\ \hline
Hydrophobic Moment $\alpha$ & 1 \\ \hline
Hydrophobic Moment $\beta$ & 1 \\ \hline
Hydrophobicity & 1 \\ \hline
Instability Index & 1 \\ \hline
Isoelectric Point & 1 \\ \hline
Mass Shift & 1 \\ \hline
Molecular Weight & 1 \\ \hline
Mass over charge ratio & 1 \\ \hline
\hline
Total length  & 13 \\  \hline                                               
\end{tabular}
\label{table:properties_list}
\end{table}

%%%%%%%%%%%%%%%%%%%%%%%%%%%%%%%%%%%%%%%%%%%%%%%%%%%%%%%
\end{document} %%%%%%%%%%%%%%%%%%%%%%%%%%%%%%%%%%%%%%%%
